# Supplementary material for: Communication, and concurrency with logic-based restriction inside a calculus of structures
Source: arXiv:1212.4669 source file (2012-12-19)
Supplement: Supplementary file 1 [file Appendix-Partial-Completeness-BVTL-BVT.tex]

\section{Proof of \textit{Big-step commuting conversions in $ \BVT $}
(Proposition~\ref{proposition:Big-step commuting conversions in BVT},
page~\pageref{proposition:Big-step commuting conversions in BVT})}
\label{section:Proof of proposition:Big-step commuting conversions in BVT}
%%%%%%%%%
We apply Point~\ref{enum:Splitting-seq} of Theorem~\ref{theorem:Splitting-ALT} to the part of $ \bvtPder  $ that includes $ \bvtPder'$ and $ (*) $ for which we forcefully have
$\vlstore{\strFN{\vlsbr<\strT;\strS''[\atma;\natma]>}
 \cap\strBN{\vlsbr<\strT;\strS''[\atma;\natma]>}=\emptyset}
 \vlread$. There are $\strK_1, \strK_2$, and, possibly, some atoms
$\vec{\atmb}$ \ST:
{\small
$$
\vlderivation{
\vlde{\bvtEder}{\BVT}
     {\strS'
      \vlsbr<\strT;\strS''[\atma;\natma]>}{
\vlhy{\vlfo{\vec{\atmb}}
           {\vlsbr[\vlsbr<\strT;\strS''[\atma;\natma]>
                  ;\strK_1;\strK_2]}}}}
\qquad
\vlderivation{
\vlpd{\bvtQder'}{\BVT}
     {\vlsbr[\strT;\strK_1]}}
\qquad
\vlderivation{
\vlpd{\bvtQder''}{\BVT}
     {\vlsbr[\strS''[\atma;\natma];\strK_2]}}
     $$
}%\small
\noindent
We observe that $\bvtQder''$ can always be of the form:
{\small
$$
\vlderivation{
\vlin{\bvtatidrule}{}
     {\vlsbr[\strS''[\atma;\natma];\strK_2]} {
\vlpd{\bvtQder'''}{\BVT}
     {\vlsbr[\strS''\,\vlscn{\vlone};\strK_2]}}}
$$
} %\small
\noindent
just because no constraint exists to annihilate the occurrence of $\atma$, and of $\natma$ in $\strS''\vlhole$.
We compose all the derivations, and proof outlined so far:
{\small
$$
\vlderivation{
\vlde{\bvtDder'}{\BVT}
     {\strR}{
\vlde{\bvtEder}{\BVT}
     {\strS'
      \vlsbr<\strT;\strS''[\atma;\natma]>}{
\vlin{\bvtseqdrule}{}
     {\vlfo{\vec{\atmb}}
           {\vlsbr
            [<\strT;\strS''[\atma;\natma]>
            ;\strK_1;\strK_2]}}{
\vlde{\bvtQder'}{\BVT}
     {\vlfo{\vec{\atmb}}
           {\vlsbr
            <[\strT;\strK_1]
             ;[\strS''[\atma;\natma]
              ;\strK_2]>}
     }{
\vlin{\bvtatidrule}{(**)}
     {\vlfo{\vec{\atmb}}
           {\vlsbr
            [\strS''[\atma;\natma]
              ;\strK_2]}
     }{
\vlpr{\bvtQder'''}{\BVT}
     {\vlfo{\vec{\atmb}}
           {\vlsbr
            [\strS''\,\vlscn{\vlone}
              ;\strK_2]}
     }}}}}}}
     $$
}%\small
The resulting proof contains $(**)$ whose \OpNameSeq-number
is strictly smaller than the one of $(*)$.
